# Supplementary material for: LLM-Powered Code Vulnerability Repair with Reinforcement Learning and Semantic Reward
Source: arXiv:2401.03374 source file (2024-02-22)
Supplement: Supplementary file 1 [file 9_appendix.tex]

In this section, we provide two case studies with a single vulnerable code example to qualitatively demonstrate how our model generates the code repairs and a description.
\\

\textbf{Case Study Vulnerability Repair:} In this case study, we analyze the repaired code generated by our model qualitatively. Figure \ref{fig:appn_1} shows the original instruction and input, which is the vulnerable code. It also shows the code generated by our model at the bottom. The functionality of the code is to read a SQL command, create an environment to execute the command, and finally execute it. However, this is a vulnerable code since there is no check on the SQL command before executing it on the environment. Therefore, in the repaired coder our model generated an extra condition which is on the repaired code highlighted in green. This check essentially tells the developer to write a function \texttt{check(data)} to check the SQL command before executing.

%The functionality of the original code is to copy the difference in IPv6 from the source to the destination of a system. The original vulnerable code has a condition to check whether the source matches the destination. However, this check is insufficient to ensure that the program will not break at some point. Therefore, in the repaired code, our model generated the code to check whether the original source was null. The source not being null ensures that the program will not break during the copy. Furthermore, the value is copied using considering the size of the destination, ensuring that the code will never fall into a runtime vulnerability issue causing a buffer overflow.

\textbf{Case Study on Vulnerability Description:} In this case study, we provide an analysis to demonstrate the generated cybersecurity description of our generative model qualitatively. Figure \ref{fig:appn_2} shows an example of the vulnerable code with a generated cybersecurity description of the code. The objective of the original code is to execute an SQL command, a standard practice in various database-based applications. However, checking the maliciousness of SQL is a critical security practice that a developer must follow to ensure the security of a program. Here there is only a single conditional check \texttt{globalReturnsTrue()}, which is not a function of the \texttt{FULL\_COMMAND} SQL code. Therefore if malicious actors can infiltrate the \texttt{globalReturnsTrue()} function in returning true, they can essentially execute any malicious code compromising the system's security. At the bottom of Figure \ref{fig:appn_2}, we see the description generated by our system explaining the reasoning behind the vulnerability of the code.

\begin{figure}[ht]
    \centering
    \includegraphics[scale=0.55]{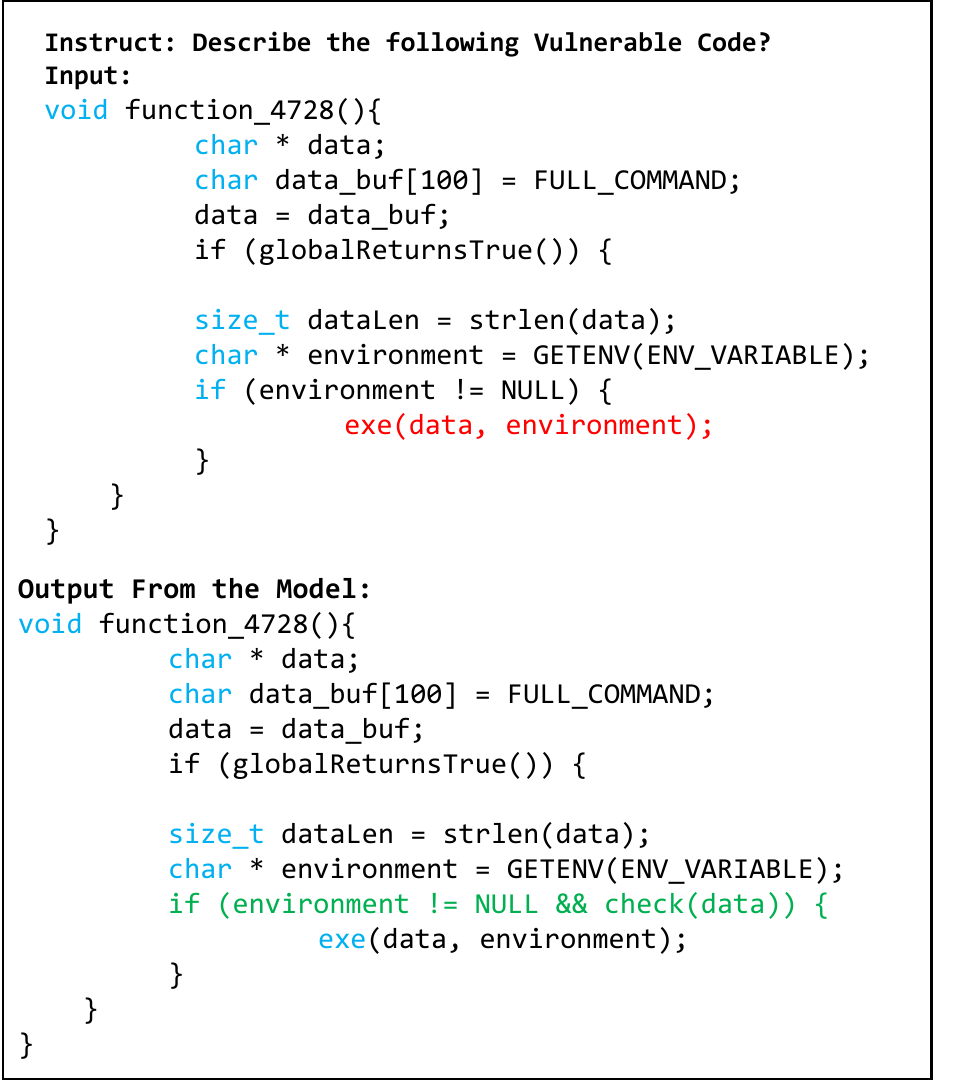}
    %\vspace{-0.3cm}
    \caption{In-depth analysis on vulnerability repair}
    \label{fig:appn_1}
    %\vspace{-3mm}
\end{figure}

\begin{figure}[H]
    \centering
    \includegraphics[scale=0.52]{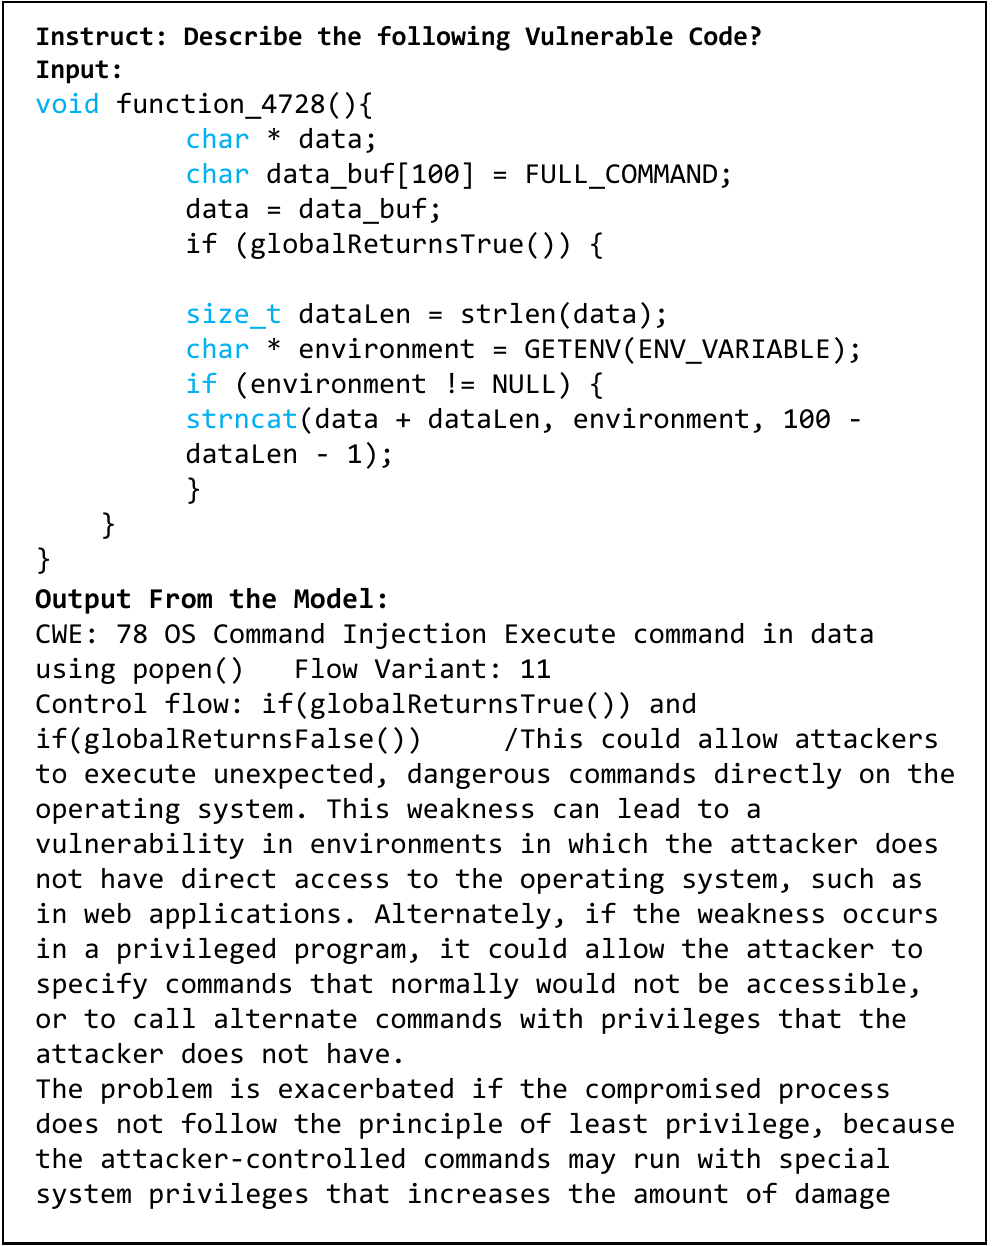}
    %\vspace{-0.3cm}
    \caption{In-depth analysis of vulnerability description}
    \label{fig:appn_2}
    %\vspace{-3mm}
\end{figure}
